# Supplementary material for: Hybridized Discontinuous Galerkin Methods for a Multiple Network Poroelasticity Model with Medical Applications
Source: arXiv:2205.06732 source file (2022-05-13)
Supplement: Supplementary file 1 [file abs_u_mean.tex]

% This file was created with tikzplotlib v0.9.15.
\definecolor{color0}{rgb}{0.12156862745098,0.466666666666667,0.705882352941177}
\definecolor{color1}{rgb}{1,0.498039215686275,0.0549019607843137}
\definecolor{color2}{rgb}{0.172549019607843,0.627450980392157,0.172549019607843}

\begin{axis}[
legend cell align={left},
legend style={
  fill opacity=0.8,
  draw opacity=1,
  text opacity=1,
  at={(0.03,0.97)},
  anchor=north west,
  draw=white!80!black
},
tick align=outside,
tick pos=left,
x grid style={white!69.0196078431373!black},
xlabel={t},
xmin=-124.8, xmax=2620.8,
xtick style={color=black},
y grid style={white!69.0196078431373!black},
ymin=0.000712324741880971, ymax=0.0670761413797702,
ytick style={color=black}
]
\addplot [semithick, color0]
table {%
0 0.00372886186178503
8 0.00390762440836921
16 0.00390757181027335
24 0.00390732528176923
32 0.00390711189776396
40 0.00394222744041536
48 0.00399114742886245
56 0.0040386235940449
64 0.00408473546307875
72 0.00412954805261623
80 0.00417311519422769
88 0.00421548237437134
96 0.004256688915913
104 0.00429676961721495
112 0.00433575609240974
120 0.00437367798182608
128 0.00441056430604
136 0.00444644559921285
144 0.00448135867308724
152 0.00451536177003684
160 0.00454860771120384
168 0.00458213533951668
176 0.00462990489398265
184 0.00468902502729242
192 0.0047473334536063
200 0.00480410564858061
208 0.00485927050280003
216 0.00491283696399236
224 0.00496483492662601
232 0.0050153041204699
240 0.00506429470404139
248 0.00511187977424967
256 0.00515821286827694
264 0.0052039386470958
272 0.00525470027561549
280 0.00531491330715244
288 0.00537522198126299
296 0.00543397060893477
304 0.00549098229533582
312 0.00554624815135789
320 0.00559979668007433
328 0.00565166827340701
336 0.00570190811815804
344 0.00575056390475143
352 0.00579768557529005
360 0.00584332621109615
368 0.00588754500647269
376 0.00593041450608269
384 0.00597204014154878
392 0.00601262157054547
400 0.00605268023429079
408 0.00609376511989311
416 0.00613762982685415
424 0.0061826092968138
432 0.00622697116500829
440 0.00627018546263324
448 0.00631211432539878
456 0.00635273114957675
464 0.00639204689069233
472 0.00643008707850675
480 0.00646688347706268
488 0.00650247042859819
496 0.00653688326351075
504 0.0065701573945926
512 0.00660232793115496
520 0.00663342940239998
528 0.00666349559452797
536 0.00669255948719943
544 0.00672065322482385
552 0.00674780809451726
560 0.00677405447354444
568 0.00679942189665324
576 0.00682393902024753
584 0.00684763364581352
592 0.00687053271733054
600 0.00689266239133961
608 0.00691404799255371
616 0.00693471406583304
624 0.00695468439848855
632 0.0069739820152227
640 0.00699262922393589
648 0.007010647623096
656 0.00702805810434254
664 0.00704488092924526
672 0.0070611356670789
680 0.00707684128273506
688 0.00709201611356691
696 0.00710667791500647
704 0.00712084384759575
712 0.00713453052999532
720 0.00714775402588919
728 0.00716052987375856
736 0.00717287311229822
744 0.00718479826861803
752 0.0071963194101962
760 0.00720745012580004
768 0.00721820355695341
776 0.00722859242214245
784 0.00723862898516843
792 0.00724832515044949
800 0.00725769239538707
808 0.00726674181512702
816 0.00727548415405619
824 0.0072839297740588
832 0.00729208869564453
840 0.00729997063955024
848 0.00730758495250994
856 0.0073149406847917
864 0.00732204659661215
872 0.00732891114061574
880 0.00733554249644265
888 0.00734194855993867
896 0.00734813695062301
904 0.00735411506838626
912 0.00735989001869972
920 0.00736546869208777
928 0.00737085775999761
936 0.00737606363739074
944 0.00738109254759267
952 0.00738595050019788
960 0.00739064328076819
968 0.00739517649751123
976 0.00739955558629198
984 0.00740378575383655
992 0.00740787207390592
1000 0.00741181941977865
1008 0.00741563252289805
1016 0.00741931593763267
1024 0.00742287406672975
1032 0.00742631117533817
1040 0.007429631364996
1048 0.00743283862354286
1056 0.00743593677633222
1064 0.00743892953116343
1072 0.00744182047516722
1080 0.00744461306881001
1088 0.00744731065820711
1096 0.00744991645927033
1104 0.00745243361456594
1112 0.00745486511788253
1120 0.0074572139031299
1128 0.00745948275147527
1136 0.00746167442348813
1144 0.00746379150991144
1152 0.00746583656394429
1160 0.00746781201985628
1168 0.00746972027098584
1176 0.00747156357059955
1184 0.00747334415204715
1192 0.00747506414638069
1200 0.00747672560676869
1208 0.00747833052897862
1216 0.00747988083483875
1224 0.00748137839020887
1232 0.00748282497506
1240 0.00748422232737416
1248 0.0074855721326908
1256 0.00748687600235179
1264 0.00748813549630416
1272 0.00748935213367218
1280 0.00749052735782296
1288 0.00749166258932918
1296 0.0074927591911383
1304 0.00749381846935651
1312 0.00749484169893536
1320 0.00749583009809711
1328 0.00749678487267731
1336 0.0074977071440042
1344 0.00749859803074479
1352 0.00749945860396007
1360 0.00750028988443555
1368 0.00750109286874004
1376 0.00750186852476369
1384 0.00750261779420678
1392 0.00750334155780034
1400 0.00750404068441434
1408 0.00750471602253639
1416 0.00750536837433763
1424 0.00750599853226061
1432 0.00750660722962082
1440 0.00750719522273008
1448 0.00750776320128337
1456 0.00750831184665261
1464 0.00750884182787491
1472 0.00750935376308537
1480 0.00750984828588096
1488 0.00751032596552109
1496 0.00751078740338988
1504 0.00751123312402765
1512 0.00751166368124987
1520 0.00751207958785759
1528 0.00751248133573438
1536 0.0075128694054854
1544 0.00751324427695793
1552 0.00751360639221972
1560 0.00751395617721036
1568 0.00751429406311621
1576 0.00751462044419981
1584 0.00751493572682459
1592 0.0075152402719128
1600 0.00751553445555763
1608 0.00751581862292399
1616 0.00751609312348686
1624 0.00751635828517561
1632 0.00751661441531663
1640 0.00751686183367096
1648 0.00751710083331252
1656 0.00751733169536611
1664 0.00751755470825091
1672 0.00751777012156852
1680 0.00751797820754784
1688 0.00751817921101735
1696 0.0075183733806471
1704 0.0075185609349224
1712 0.00751874210925567
1720 0.00751891712241989
1728 0.00751908617247842
1736 0.00751924947112528
1744 0.00751940721235873
1752 0.00751955958897853
1760 0.00751970677625444
1768 0.00751984895936693
1776 0.00751998629876669
1784 0.00752011897168166
1792 0.00752024710871865
1800 0.00752037091372178
1808 0.0075204904919259
1816 0.00752060600278189
1824 0.00752071757880806
1832 0.0075208253585417
1840 0.00752092947383541
1848 0.00752103004021885
1856 0.00752112718967659
1864 0.00752122103365032
1872 0.00752131167982175
1880 0.00752139924542717
1888 0.00752148383084267
1896 0.00752156554549879
1904 0.00752164447129317
1912 0.00752172070476432
1920 0.00752179434612578
1928 0.00752186548722197
1936 0.00752193420348118
1944 0.00752200059020444
1952 0.00752206470306716
1960 0.00752212664165949
1968 0.00752218647445374
1976 0.00752224426666906
1984 0.00752230009646645
1992 0.00752235402726415
2000 0.00752240612060083
2008 0.00752245644472556
2016 0.0075225050505048
2024 0.00752255200482154
2032 0.00752259736142117
2040 0.00752264117369608
2048 0.00752268349175751
2056 0.0075227243752675
2064 0.00752276386427347
2072 0.00752280201014473
2080 0.00752283886364642
2088 0.0075228744609984
2096 0.00752290884261166
2104 0.00752294205370901
2112 0.00752297413305263
2120 0.00752300513019222
2128 0.00752303507212356
2136 0.00752306398264169
2144 0.00752309192433735
2152 0.0075231189032825
2160 0.00752314496771007
2168 0.00752317015391861
2176 0.00752319446694832
2184 0.00752321796115432
2192 0.00752324065319577
2200 0.00752326258088465
2208 0.00752328375802386
2216 0.0075233042130633
2224 0.00752332397758199
2232 0.0075233430661749
2240 0.00752336149962883
2248 0.00752337930985788
2256 0.00752339651284987
2264 0.00752341313423912
2272 0.00752342918787557
2280 0.00752344469290278
2288 0.00752345967627483
2296 0.00752347414629967
2304 0.00752348812304366
2312 0.00752350162310644
2320 0.00752351466170522
2328 0.00752352726131654
2336 0.00752353943284442
2344 0.007523551192892
2352 0.00752356254791695
2360 0.00752357351153321
2368 0.0075235841101462
2376 0.00752359434456987
2384 0.0075236042360669
2392 0.00752361378613598
2400 0.00752362300962553
2408 0.00752363192170303
2416 0.00752364052854119
2424 0.00752364884413899
2432 0.007523656879548
2440 0.00752366464027381
2448 0.00752367213900011
2456 0.00752367937214749
2464 0.00752368636983449
2472 0.00752369312406437
2480 0.00752369964370429
2488 0.00752370595642953
2496 0.0075237120399538
};
\addlegendentry{$P_1$}
\addplot [semithick, color1]
table {%
0 0.0323727087347629
8 0.0338933670671431
16 0.03389294006611
24 0.0338920967472139
32 0.0339020134356809
40 0.0341960514306375
48 0.0346075311008806
56 0.0350093266230883
64 0.0353998394041648
72 0.0357793636210441
80 0.0361483271799071
88 0.0365071278692894
96 0.0368561146855014
104 0.037195593035212
112 0.037525833680001
120 0.0378470814120627
128 0.0381595628653104
136 0.038463494413889
144 0.0387590927786747
152 0.0390465971781066
160 0.0393263445041957
168 0.0395992292535358
176 0.0398801073716906
184 0.0403506654051699
192 0.0408465977267312
200 0.0413295414974826
208 0.0417987608600051
216 0.0422543963035717
224 0.0426967378848337
232 0.04312613783121
240 0.0435430125134396
248 0.0439479000013394
256 0.0443416521633644
264 0.0447261830616536
272 0.0451086745648309
280 0.0455267107857059
288 0.0460104944647506
296 0.0465032460930107
304 0.0469856990870576
312 0.0474547007637885
320 0.0479096763558567
328 0.0483506645409014
336 0.0487779023100402
344 0.0491917037508376
352 0.0495924164519301
360 0.0499804041896407
368 0.0503560404840054
376 0.0507197087880233
384 0.0510718096161754
392 0.0514127807030588
400 0.0517431509597021
408 0.0520637053712979
416 0.0523761218834257
424 0.0526862978545216
432 0.0530160019496805
440 0.0533705920831952
448 0.0537245751986114
456 0.0540697431753221
464 0.0544045509222168
472 0.0547287662787074
480 0.0550425030942201
488 0.0553459903646325
496 0.0556394999528087
504 0.0559233194441657
512 0.0561977403372793
520 0.0564630525295417
528 0.0567195415311375
536 0.0569674869447414
544 0.0572071617267211
552 0.057438831693925
560 0.0576627554699078
568 0.0578791842876621
576 0.0580883621211021
584 0.0582905257094287
592 0.0584859046943543
600 0.0586747217144555
608 0.0588571926000262
616 0.0590335264932124
624 0.0592039260125807
632 0.0593685874273523
640 0.059527700817134
648 0.0596814502428098
656 0.0598300139206423
664 0.0599735643301868
672 0.0601122684555594
680 0.0602462878993669
688 0.0603757790360825
696 0.0605008931806836
704 0.0606217767328068
712 0.0607385713243258
720 0.0608514139741097
728 0.0609604372025639
736 0.061065769200443
744 0.0611675339342011
752 0.0612658513015087
760 0.0613608372340665
768 0.0614526038549768
776 0.0615412595432926
784 0.0616269091502315
792 0.0617096539661446
800 0.0617895919801279
808 0.0618668179043973
816 0.0619414232798152
824 0.0620134966160612
832 0.062083123472126
840 0.0621503865118907
848 0.0622153656783977
856 0.0622781382228493
864 0.0623387787963727
872 0.062397359580383
880 0.0624539502725598
888 0.0625086182896955
896 0.0625614287650887
904 0.0626124446322379
912 0.0626617267231365
920 0.062709333800095
928 0.0627553226646313
936 0.062799748200137
944 0.0628426634253836
952 0.0628841195806578
960 0.062924166185067
968 0.0629628510838987
976 0.0630002204775477
984 0.0630363190532448
992 0.0630711899348717
1000 0.0631048748325454
1008 0.0631374140211103
1016 0.0631688464196315
1024 0.0631992096231043
1032 0.0632285399581637
1040 0.0632568725262907
1048 0.0632842412282424
1056 0.0633106788192102
1064 0.0633362169586397
1072 0.0633608862146538
1080 0.0633847161217714
1088 0.0634077352149008
1096 0.0634299710733808
1104 0.0634514503102159
1112 0.0634721986678847
1120 0.0634922409866786
1128 0.0635116013035723
1136 0.0635303027792502
1144 0.0635483678445996
1152 0.0635658181461449
1160 0.0635826745921659
1168 0.0635989573677236
1176 0.0636146860169406
1184 0.0636298793739055
1192 0.0636445556501882
1200 0.0636587324443267
1208 0.063672426740089
1216 0.0636856549597529
1224 0.063698432960393
1232 0.0637107760705425
1240 0.0637226990806532
1248 0.0637342162795839
1256 0.0637453414899731
1264 0.0637560880387718
1272 0.0637664688132701
1280 0.0637764962713964
1288 0.0637861824305974
1296 0.0637955389033846
1304 0.0638045769151222
1312 0.063813307298676
1320 0.0638217405301294
1328 0.0638298867154457
1336 0.0638377556321812
1344 0.0638453567061594
1352 0.0638526990637455
1360 0.0638597915055154
1368 0.0638666425432833
1376 0.0638732603950388
1384 0.0638796529761113
1392 0.0638858279812889
1400 0.0638917927973888
1408 0.0638975545912649
1416 0.0639031202665185
1424 0.0639084964974916
1432 0.0639136897417524
1440 0.0639187062146302
1448 0.0639235519414021
1456 0.0639282327312262
1464 0.0639327541924938
1472 0.0639371217696533
1480 0.0639413406713033
1488 0.0639454159864541
1496 0.0639493525787567
1504 0.0639531551872925
1512 0.0639568283608872
1520 0.0639603765136154
1528 0.0639638038913201
1536 0.0639671146193297
1544 0.0639703126596751
1552 0.0639734018463105
1560 0.0639763858850315
1568 0.0639792683593992
1576 0.0639820527228517
1584 0.0639847423092971
1592 0.0639873403683685
1600 0.0639898499861589
1608 0.0639922741837957
1616 0.0639946158748807
1624 0.0639968778633421
1632 0.0639990628659315
1640 0.0640011735004531
1648 0.0640032122850372
1656 0.0640051816911237
1664 0.0640070840601234
1672 0.0640089216783237
1680 0.0640106967574376
1688 0.0640124114220707
1696 0.0640140677278373
1704 0.0640156676461788
1712 0.0640172131290775
1720 0.0640187059954306
1728 0.0640201480621139
1736 0.0640215410492408
1744 0.0640228866221742
1752 0.0640241863959155
1760 0.0640254419406175
1768 0.0640266547414357
1776 0.0640278262716108
1784 0.0640289579254811
1792 0.0640300510844035
1800 0.0640311070012749
1808 0.0640321270057692
1816 0.0640331122906748
1824 0.0640340640433459
1832 0.0640349833978332
1840 0.0640358714675688
1848 0.0640367293160819
1856 0.0640375579659392
1864 0.0640383584097163
1872 0.0640391316135106
1880 0.0640398785077437
1888 0.0640405999757103
1896 0.0640412968804817
1904 0.0640419700834426
1912 0.0640426203748869
1920 0.0640432485281492
1928 0.0640438553024767
1936 0.0640444414303082
1944 0.0640450076047045
1952 0.0640455545187224
1960 0.064046082815049
1968 0.0640465931395759
1976 0.0640470860852385
1984 0.0640475622580193
1992 0.0640480222275499
2000 0.0640484665429027
2008 0.0640488957312031
2016 0.0640493103223702
2024 0.0640497107995746
2032 0.0640500976448874
2040 0.064050471325667
2048 0.0640508322962722
2056 0.0640511809756759
2064 0.0640515177912927
2072 0.0640518431444183
2080 0.0640521574235072
2088 0.0640524610060642
2096 0.0640527542608684
2104 0.0640530375369917
2112 0.064053311170432
2120 0.0640535754862565
2128 0.0640538308065111
2136 0.0640540774505709
2144 0.0640543156834849
2152 0.0640545458229668
2160 0.064054768129466
2168 0.0640549828595732
2176 0.0640551902958155
2184 0.0640553906687854
2192 0.0640555842229173
2200 0.0640557711850221
2208 0.0640559517877059
2216 0.0640561262472321
2224 0.064056294757812
2232 0.0640564575416214
2240 0.0640566147953151
2248 0.0640567666903337
2256 0.0640569134094296
2264 0.0640570551440717
2272 0.0640571920540464
2280 0.0640573243039453
2288 0.0640574520488041
2296 0.0640575754508619
2304 0.064057694654497
2312 0.0640578098012216
2320 0.0640579210342187
2328 0.064058028472456
2336 0.0640581322597558
2344 0.0640582325074381
2352 0.0640583293492324
2360 0.0640584229029844
2368 0.064058513263218
2376 0.0640586005578203
2384 0.0640586848680267
2392 0.0640587663115321
2400 0.0640588449928225
2408 0.0640589209966882
2416 0.0640589944090072
2424 0.0640590653282457
2432 0.0640591338246447
2440 0.0640592000040266
2448 0.0640592639128686
2456 0.0640593256606889
2464 0.0640593852971217
2472 0.0640594429160111
2480 0.0640594985680794
2488 0.0640595523228443
2496 0.0640596042598661
};
\addlegendentry{$P_2$}
\addplot [semithick, color2]
table {%
0 0.0218198348686629
8 0.0228288389827851
16 0.0228285327727882
24 0.0228272212966187
32 0.0228281126996722
40 0.023054433366921
48 0.023337935370182
56 0.0236134011723342
64 0.0238810851213953
72 0.0241413415561642
80 0.0243944746830613
88 0.0246407393125925
96 0.0248803515744474
104 0.0251134984985819
112 0.0253403455794259
120 0.0255610423993007
128 0.0257757270372502
136 0.0259845292544631
144 0.0261875728895667
152 0.0263849776603031
160 0.0265768607047678
168 0.0267633382287522
176 0.0269911035470963
184 0.0273434432187513
192 0.027685636214671
200 0.0280179019057092
208 0.028340466763917
216 0.0286535605785865
224 0.0289574195033142
232 0.02925229319575
240 0.029538463378361
248 0.0298163008739858
256 0.0300865017802675
264 0.0303517498705321
272 0.0306411033936014
280 0.030993010174162
288 0.0313460463885842
296 0.0316897160148108
304 0.0320231232804139
312 0.0323462671166674
320 0.0326593317890963
328 0.0329625570680495
336 0.0332562024762436
344 0.0335405351495666
352 0.0338158256631441
360 0.0340823480042776
368 0.0343403832633211
376 0.0345902303930944
384 0.0348322358830305
392 0.0350668886067184
400 0.035295222181534
408 0.0355214471870244
416 0.0357658599198396
424 0.0360298062010667
432 0.0362910555220409
440 0.0365450693617088
448 0.0367912023246156
456 0.0370294421787847
464 0.0372599351694394
472 0.0374828781077301
480 0.0376984850472829
488 0.0379069747978319
496 0.0381085655832993
504 0.0383034725364437
512 0.0384919064306562
520 0.0386740730658894
528 0.0388501729175413
536 0.0390204010564557
544 0.0391849470090029
552 0.0393439948940275
560 0.039497723349893
568 0.039646305783227
576 0.0397899102877517
584 0.0399286998913856
592 0.040062832604908
600 0.040192461558646
608 0.040317735092362
616 0.0404387969473681
624 0.0405557862924257
632 0.0406688379583716
640 0.0407780824600758
648 0.0408836461605843
656 0.0409856513835323
664 0.0410842165323572
672 0.0411794562085656
680 0.0412714812701596
688 0.0413603990471967
696 0.0414463133382653
704 0.0415293246055464
712 0.0416095299823829
720 0.041687023478486
728 0.041761895997101
736 0.0418342354430376
744 0.0419041268919198
752 0.0419716525407363
760 0.0420368919333424
768 0.0420999219457277
776 0.0421608169421854
784 0.04221964880656
792 0.0422764870416354
800 0.0423313988157204
808 0.042384449113444
816 0.0424357007064732
824 0.0424852143131599
832 0.0425330486125363
840 0.0425792602880384
848 0.0426239041867051
856 0.0426670332874616
864 0.0427086988086315
872 0.042748950211241
880 0.0427878353855818
888 0.0428254005182736
896 0.0428616903167752
904 0.0428967479098585
912 0.0429306150599756
920 0.0429633321032548
928 0.0429949379468389
936 0.043025470281195
944 0.0430549654741176
952 0.0430834586786718
960 0.0431109838831141
968 0.043137573900074
976 0.0431632604299138
984 0.0431880741404134
992 0.0432120446373071
1000 0.0432352005243556
1008 0.0432575694426042
1016 0.0432791780947889
1024 0.0433000522855585
1032 0.0433202169621259
1040 0.0433396961921464
1048 0.0433585132465304
1056 0.0433766906364902
1064 0.043394250060954
1072 0.0434112125082892
1080 0.0434275982587284
1088 0.0434434268933492
1096 0.0434587173581569
1104 0.0434734879101201
1112 0.0434877562410826
1120 0.0435015393846955
1128 0.0435148538484976
1136 0.0435277155304501
1144 0.0435401398657602
1152 0.0435521416608045
1160 0.0435637353316502
1168 0.0435749347036687
1176 0.043585753212444
1184 0.0435962037840506
1192 0.0436062989264538
1200 0.0436160507229574
1208 0.0436254708540437
1216 0.0436345706003868
1224 0.04364336082449
1232 0.0436518520784478
1240 0.0436600545289189
1248 0.0436679779770153
1256 0.0436756319073725
1264 0.0436830255054942
1272 0.043690167612414
1280 0.04369706677735
1288 0.0437037312751575
1296 0.0437101690563402
1304 0.0437163878513826
1312 0.0437223951142495
1320 0.0437281980369908
1328 0.0437338035430706
1336 0.0437392183800283
1344 0.0437444490157523
1352 0.0437495017036314
1360 0.0437543825286455
1368 0.0437590973132242
1376 0.0437636517010655
1384 0.0437680511595291
1392 0.0437723009527829
1400 0.0437764061886042
1408 0.0437803717454361
1416 0.0437842024103591
1424 0.043787902742849
1432 0.0437914772201942
1440 0.0437949300765745
1448 0.0437982654634362
1456 0.0438014873938537
1464 0.0438045997096215
1472 0.0438076061347135
1480 0.0438105102862155
1488 0.0438133156488639
1496 0.043816025550434
1504 0.043818643274131
1512 0.0438211719376731
1520 0.0438236145709708
1528 0.0438259741099584
1536 0.04382825338492
1544 0.0438304550960863
1552 0.0438325818998937
1560 0.0438346363637749
1568 0.0438366209211135
1576 0.0438385379760803
1584 0.0438403897969701
1592 0.0438421786121585
1600 0.0438439065789478
1608 0.0438455757680639
1616 0.0438471881508544
1624 0.0438487456794571
1632 0.0438502502248397
1640 0.0438517035773112
1648 0.0438531074930754
1656 0.0438544636315579
1664 0.0438557736315038
1672 0.0438570390833258
1680 0.0438582614640101
1688 0.0438594422609538
1696 0.0438605828693016
1704 0.0438616847098218
1712 0.0438627490259126
1720 0.0438637771494238
1728 0.0438647702916244
1736 0.0438657296407986
1744 0.043866656353659
1752 0.0438675515452939
1760 0.0438684162677419
1768 0.0438692515728265
1776 0.043870058462115
1784 0.0438708378945617
1792 0.043871590814879
1800 0.0438723181252529
1808 0.0438730206711001
1816 0.0438736993201637
1824 0.0438743548841788
1832 0.043874988157708
1840 0.0438755998639112
1848 0.0438761907698982
1856 0.0438767615619382
1864 0.043877312941043
1872 0.0438778455668814
1880 0.0438783600557613
1888 0.0438788570516905
1896 0.0438793371352256
1904 0.04387980087358
1912 0.0438802488481494
1920 0.0438806815953343
1928 0.0438810995977106
1936 0.0438815033891894
1944 0.0438818934307675
1952 0.0438822702158782
1960 0.0438826341811368
1968 0.0438829857356903
1976 0.0438833253628096
1984 0.0438836534222969
1992 0.0438839703072474
2000 0.043884276425277
2008 0.0438845721268122
2016 0.0438848577662524
2024 0.0438851336819831
2032 0.0438854002239735
2040 0.0438856576943648
2048 0.0438859064019236
2056 0.0438861466459582
2064 0.0438863787138178
2072 0.0438866028864089
2080 0.0438868194243882
2088 0.0438870286106529
2096 0.0438872306709595
2104 0.043887425861318
2112 0.0438876144115156
2120 0.0438877965395536
2128 0.0438879724720288
2136 0.0438881424248653
2144 0.0438883065891118
2152 0.0438884651758783
2160 0.0438886183557257
2168 0.0438887663323379
2176 0.0438889092764428
2184 0.043889047349766
2192 0.0438891807279496
2200 0.0438893095623053
2208 0.0438894340205481
2216 0.0438895542368895
2224 0.0438896703834342
2232 0.0438897825569191
2240 0.0438898909140086
2248 0.0438899955927832
2256 0.043890096718947
2264 0.0438901943859167
2272 0.0438902887368448
2280 0.043890379881275
2288 0.0438904679177885
2296 0.0438905529595808
2304 0.0438906351166543
2312 0.0438907144716045
2320 0.0438907911275273
2328 0.0438908651791178
2336 0.0438909367060401
2344 0.0438910058007701
2352 0.0438910725432858
2360 0.043891137017919
2368 0.0438911993005146
2376 0.0438912594532142
2384 0.0438913175721292
2392 0.0438913737153353
2400 0.0438914279462287
2408 0.0438914803145612
2416 0.0438915309200985
2424 0.0438915797930232
2432 0.0438916270086663
2440 0.0438916726009639
2448 0.0438917166650122
2456 0.0438917592361601
2464 0.0438918003457237
2472 0.0438918400503209
2480 0.0438918784249596
2488 0.043891915471455
2496 0.0438919512615677
};
\addlegendentry{$P_3$}
\end{axis}
