# Supplementary material for: Hybridized Discontinuous Galerkin Methods for a Multiple Network Poroelasticity Model with Medical Applications
Source: arXiv:2205.06732 source file (2022-05-13)
Supplement: Supplementary file 2 [file table_hconv_noniso.tex]

\begin{tabular}{c|cccccc} 

$\ell \!\!\setminus \!\!| \tilde{\mathcal{T}}_h | $ &48&162&384&750&1296&2058\\
\midrule
1&44&62&67&67&68&69\\
\rowcolor{mygray}
2&69&69&70&70&68&67\\
3&71&70&65&62&58&56\\
\rowcolor{mygray}
4&66&64&58&55&52&50\\
5&61&58&53&50&48&49\\
\rowcolor{mygray}
6&59&53&50&47&45&46\\
\end{tabular}
